# Supplementary material for: Disappearance of Quasiparticles in a Bose Lattice Gas
Source: arXiv:1503.07606 ancillary file (2016-05-11)
Supplement: Supplementary file 1 [file CoolingPaperDraft_prl_SI.pdf]

# Supplemental Material for “Disappearance of Quasiparticles in a Bose Lattice Gas”

David Chen,<sup>\*</sup> Carolyn Meldgin, Philip Russ, and Brian DeMarco<sup>†</sup>

*Department of Physics, University of Illinois at Urbana-Champaign, Urbana, IL 61801, USA*

Erich Mueller

*Department of Physics, Cornell University, Ithaca, NY 14853, USA*

(Dated: May 11, 2016)

---

<sup>\*</sup> now at:Max Planck Institute of Molecular Cell Biology and Genetics, Pfotenhauerstr. 108,01307, Dresden, Germany

<sup>†</sup> bdemarco@illinois.edu

## I. EXPERIMENTAL PARAMETERS

Detailed information regarding our apparatus can be found in Ref. [1] and references therein. The geometric mean of the trap frequencies is  $\omega = 2\pi \times (55 \pm 5)$  Hz for the optical dipole trap. The atom number in the dipole trap before turning on the lattice is  $(84 \pm 4) \times 10^3$  and the temperature is  $(91 \pm 4)$  nK. The measured condensate fraction is  $N_0/N = 0.23 \pm 0.02$  before turning on the lattice. The optical lattice formed from three pairs of counter-propagating laser beams with wavelength  $\lambda = 812$  nm is turned on in 100 ms using an exponential ramp of the lattice light intensity. A 10.15 G magnetic field is applied to the atom gas to suppress spin-exchange collisions. The bandmapping procedure used for imaging transforms quasimomentum to momentum by ramping down the lattice quickly compared with  $\hbar/t$  but slowly with respect to  $\hbar/E_{\text{bg}}$ , where  $E_{\text{bg}}$  is the bandgap between the ground and first-excited bands. Quasimomentum redistribution during bandmapping can lead to a systematic error in condensate fraction [2]. For the range of condensate fraction explored here, that error is small and not dependent on condensate fraction.

For the quasimomentum relaxation measurement, the Raman beams are detuned by  $\Delta = 2\pi \times 200$  GHz from the  $D_1$  transition. The Raman beams are pulsed on for  $200 \mu\text{s}$ , and the relative frequency is swept over 1.6 kHz across a central frequency from  $\Delta\omega = \omega_1 - \omega_2 = \omega_0 + 2\pi \times (10 - 14.8)$  kHz, in correspondence to the lattice depths  $s = (4 - 8) E_R$ , where  $\omega_0 = 2\pi \times (6834.742 \pm 0.001)$  MHz is the measured bare transition frequency between  $|F = 1, m_F = 0\rangle$  and  $|2, 0\rangle$  in a 10.15 G field. Different Rabi rates are used, ranging from  $\Omega = 2\pi \times (3.2 - 4.2)$  kHz. For the cooling demonstration, the Raman beams are detuned by  $\Delta = 2\pi \times 430$  GHz and they are pulsed on for  $400 \mu\text{s}$ . The relative frequency ranges from  $\Delta\omega = \omega_0 + 2\pi \times (15.8 - 16)$  kHz and the effective Rabi rate is  $\Omega = 2\pi \times 1.0$  kHz. In both experiments, the resonant light is pulsed on for  $50 \mu\text{s}$ .

## II. QUASIMOMENTUM SELECTIVITY

In one dimension, the Raman excitation probability as function of quasimomentum is given by the formula

$$P(q_z) = \frac{\Omega^2}{\Omega^2 + \delta(q_z)^2} \sin^2 \left( \sqrt{\Omega^2 + \delta(q_z)^2} \frac{\Delta\tau}{2} \right) \quad (\text{S1})$$

where  $\Delta\tau$  is the pulse duration,  $\Omega = \Omega_1\Omega_2\langle\uparrow, n=1|e^{i\Delta kz}|\downarrow, n=0\rangle/2\Delta$  is the effective Rabi rate,  $\Omega_{1,2}$  are the Rabi rates associated with the electric dipole transition  $5S_{1/2} \rightarrow 5P_{1/2}$  for each Raman laser beam [3],  $\delta(q_z) = \omega_1 - \omega_2 - [\omega_0 + (\epsilon^{(n=1)}(q_z + \Delta q_z) - \epsilon^{(n=0)}(q_z))/\hbar]$  is the effective detuning,  $\omega_{1,2}$  are the Raman laser frequencies,  $\Delta q_z = 0.55q_B$ ,  $\epsilon^{(n=0)}(q_z)$  and  $\epsilon^{(n=1)}(q_z)$  are the tight-binding dispersion relations of the ground and first-excited bands respectively, and the frequency offset  $\omega_0$  accounts for the hyperfine splitting and Zeeman shift between the  $|\downarrow\rangle$  and  $|\uparrow\rangle$  states. Fig. S1 shows  $P(q_z)$  for the parameters used in the cooling experiment:  $\Omega = (2\pi) \times 1$  kHz,  $\Delta\omega = \omega_0 + (2\pi) \times 15.8$  kHz, and  $\Delta\tau = 0.4$  ms.

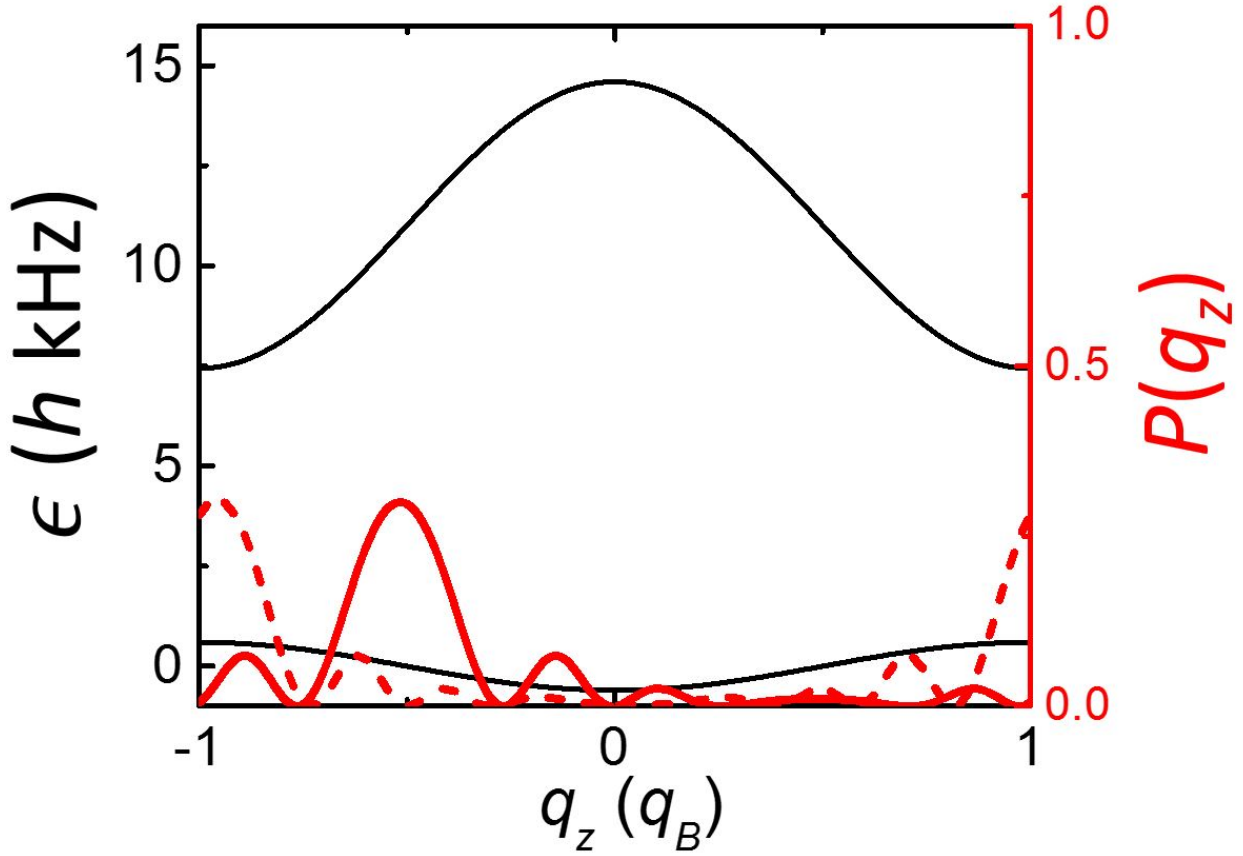

FIG. S1. Raman excitation probability for the parameters used in the cooling experiment (red-solid). The ground and first-excited bands in the tight-binding approximation are also shown as a reference (black-solid). The hyperfine splitting is not shown. A smaller  $\Delta q_z$  compared with  $q_B = \hbar\pi/d$  would permit both sides of the FBZ to be addressed simultaneously. As an example, the excitation probability for  $\Delta q_z = 0.05 q_B$  is shown as a dashed line. We ignore the weak dependence of  $\Omega$  on  $q_z$  for this calculation.

### III. IMAGE PROCESSING

The TOF images are fit to a semi-classical model that describes the equilibrium quasimomentum distribution of a non-interacting gas in a combined parabolic–lattice potential [1]. The quasimomentum distribution projected onto the imaging plane is given by

$$n(q_1, q_2) = A \sum_{i=1}^{\infty} \frac{e^{-2i\beta t(3-\cos b)} z^i}{i^{3/2}} \left( (\pi - a)I_0(\alpha_i) + 2 \sum_{j=1}^{\infty} I_j(\alpha_i) \frac{\sin j(\pi - a)}{j} \right) \quad (\text{S2})$$

where  $q_1$  and  $q_2$  are the horizontal and vertical directions in the absorption image,  $z$  is the fugacity,  $I_i$  is the modified Bessel function of the first kind,  $\alpha_j = 4j\beta t \cos a$ ,  $a = \pi|q_1 - q_1|/(2q_B)$ ,  $b = \pi(q_1 + q_2)/(\sqrt{2}q_B)$ ,  $\beta = 1/k_B T$ ,  $q_B = \hbar\pi/d$ ,  $d$  is the lattice spacing, and  $A$  is a constant. We perform the fit within a mask determined by the FBZ projected onto the imaging plane. A mask slightly smaller than the FBZ is used to account for the failure of bandmapping at the edge of the FBZ. For the rethermalization measurement, we mask out the residual condensate (corresponding to less than 6% condensate fraction) that remains in some images.

### IV. RELAXATION RATE CALCULATION

To calculate the quasimomentum relaxation rate, we consider a Maxwell-Boltzmann thermal distribution in a uniform (i.e., without a trap) lattice potential with the  $\vec{q} = 0$  atoms removed. In the relaxation-time approximation, the Boltzmann equation predicts that the number of atoms  $n_0$  at  $\vec{q} = 0$  relaxes to the equilibrium value  $n_0^{\text{eq}} = e^{-\beta(\epsilon_0 - \mu)}$  exponentially, with a time constant  $\tau_{FGR}$  given by  $\partial_t n_0 = n_0^{\text{eq}}/\tau_{FGR}$ . The time-rate-of-change  $\partial_t n_0$  is determined using Fermi's golden rule:

$$\partial_t n_0 = \frac{2U^2}{N^2} \sum_{pq} n_p n_q \frac{2\pi}{\hbar} \delta(\epsilon_{p+q} + \epsilon_0 - \epsilon_p - \epsilon_q), \quad (\text{S3})$$

where  $\epsilon_p$  is the tight-binding dispersion relation for the ground band,  $n_p = e^{-\beta(\epsilon_p - \mu)}$ ,  $\beta = 1/(k_B T)$ ,  $k_B$  is Boltzmann's constant,  $N$  is the atom number, and  $t$  and  $U$  are the Hubbard tunneling and interaction energies. The experimentally measured relaxation time  $\tau$  is given

by

$$\frac{1}{\tau} = \frac{2}{\tau_{FGR}} = \frac{4}{\hbar} n F(\beta t) \frac{U^2}{t}, \quad (\text{S4})$$

where

$$F(\beta t) = \frac{\int \frac{d^3 \vec{p}}{(2\pi)^3} \frac{d^3 \vec{q}}{(2\pi)^3} e^{2\beta t [C(\vec{p}) + C(\vec{q}) - 2C(0)]} 2\pi \delta(2C(\vec{p}) + 2C(\vec{q}) - 2C(\vec{p} + \vec{q}) - 2C(0))}{\int \frac{d^3 \vec{p}}{(2\pi)^3} e^{2\beta t [C(\vec{p}) - C(0)]}}, \quad (\text{S5})$$

$C(\vec{q}) = \sum_{i=x,y,z} \cos(q_i)$ , and  $n$  is the lattice filling. Equation S4 includes a factor of 2 for comparison to the experiment, which measures a quantity proportional to the square of the momentum-space density.

The parabolic confinement causes the lattice filling  $n$  to vary across the gas. We calculate the spatial average for  $n$  weighted by  $n$  assuming a Maxwell-Boltzmann density distribution, which results in  $\langle n \rangle = N (\beta m \omega^2 d^2 / 4\pi)^{3/2}$ . The temperature of the gas in the lattice before removing atoms for the thermalization measurement ranges from  $T = (96 - 102)$  nK. The temperature is inferred using a thermodynamic calculation and matching entropy per particle [1]. To determine  $T$  before the Raman pulse, we use the entropy per particle determined from the condensate fraction measured in the dipole trap before turning on the lattice. As shown in Fig. S2, the function  $F(\beta t) \approx 0.3$  in the regime we measure the rethermalization rate (i.e.,  $\beta t \approx 0.07 - 0.14$ ).

## V. MOMENTUM RELAXATION IN A HARMONIC TRAP

To test the method we use to measure the thermalization time in the lattice, we have measured momentum relaxation for a partially condensed gas trapped in the harmonic dipole potential. The gas is brought out of equilibrium by rapidly removing the condensate and atoms with low momentum along  $k_z$ . The remaining atoms are allowed to relax for  $t_{\text{hold}} = (0 - 100)$  ms before performing TOF imaging. We fit each image to a gaussian and calculate the mean squared residual of each fit  $r^2$  (as defined in the main text).

We observe damped oscillations in  $r^2$  with a frequency matching that of the harmonic trap (Fig.S3). The data for  $t_{\text{hold}} > 15$  ms fit well to a damped sine-squared function. We exclude the data taken at short  $t_{\text{hold}}$  when the gas is far from equilibrium from the fit, since the relaxation in that regime does not appear to be exponential. The fitted damping time constant is  $(40 \pm 10)$  ms, while the classical collision time is  $N/\Gamma = 150 \pm 40$  ms, where

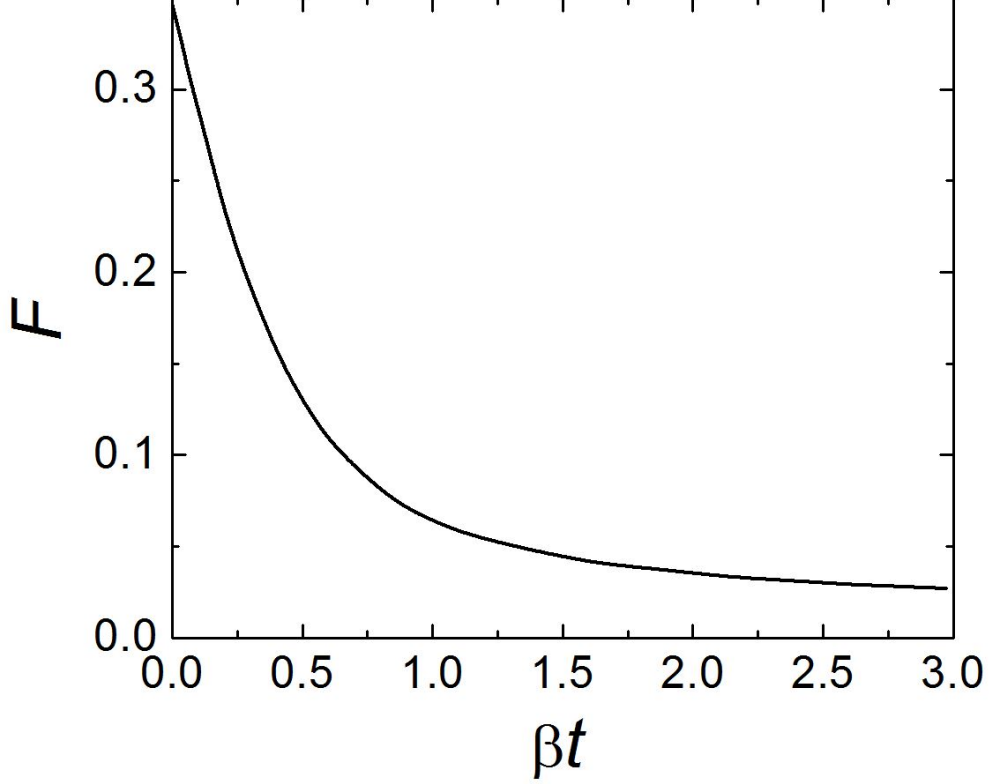

FIG. S2. Function  $F(\beta t)$  from the FGR calculation.

$\Gamma = \sigma n_{dwd} v_{rel}$  is the total collision rate,  $N$  is the atom number,  $n_{dwd} = N^2 (m\omega^2/4\pi k_B T)^{3/2}$  is the density-weighted density,  $\sigma = 8\pi a_s^2$  is the elastic collision cross section,  $a_s$  is the  $s$ -wave scattering length ( $a_s = 98a_0$  for  $^{87}\text{Rb}$ , where  $a_0$  is the Bohr radius), and  $v_{rel} = (16k_B T/\pi m)^{1/2}$  is the mean relative speed.

To compare the time constant to the collision time, we determine the average number of collisions required for rethermalization using a 3D molecular dynamics simulation of hard spheres confined in a harmonic trap. We simulate 5000 particles with an initial Maxwell-Boltzmann distribution of velocities and positions. At the beginning of the simulation, the particles with speeds 20% smaller than the average are removed along one direction. Particle trajectories are then propagated using the velocity-Verlet method. When an overlap between two particles is detected, the direction of the relative velocity is randomized (while preserving the center-of-mass velocity of the pair) to simulate  $s$ -wave collisions. The velocity distribution is analyzed at each time step to compute  $r^2$  from the equilibrium distribution. We observe behavior similar to that displayed in Fig. S3. A fit of  $r^2$  vs. the evolution time to

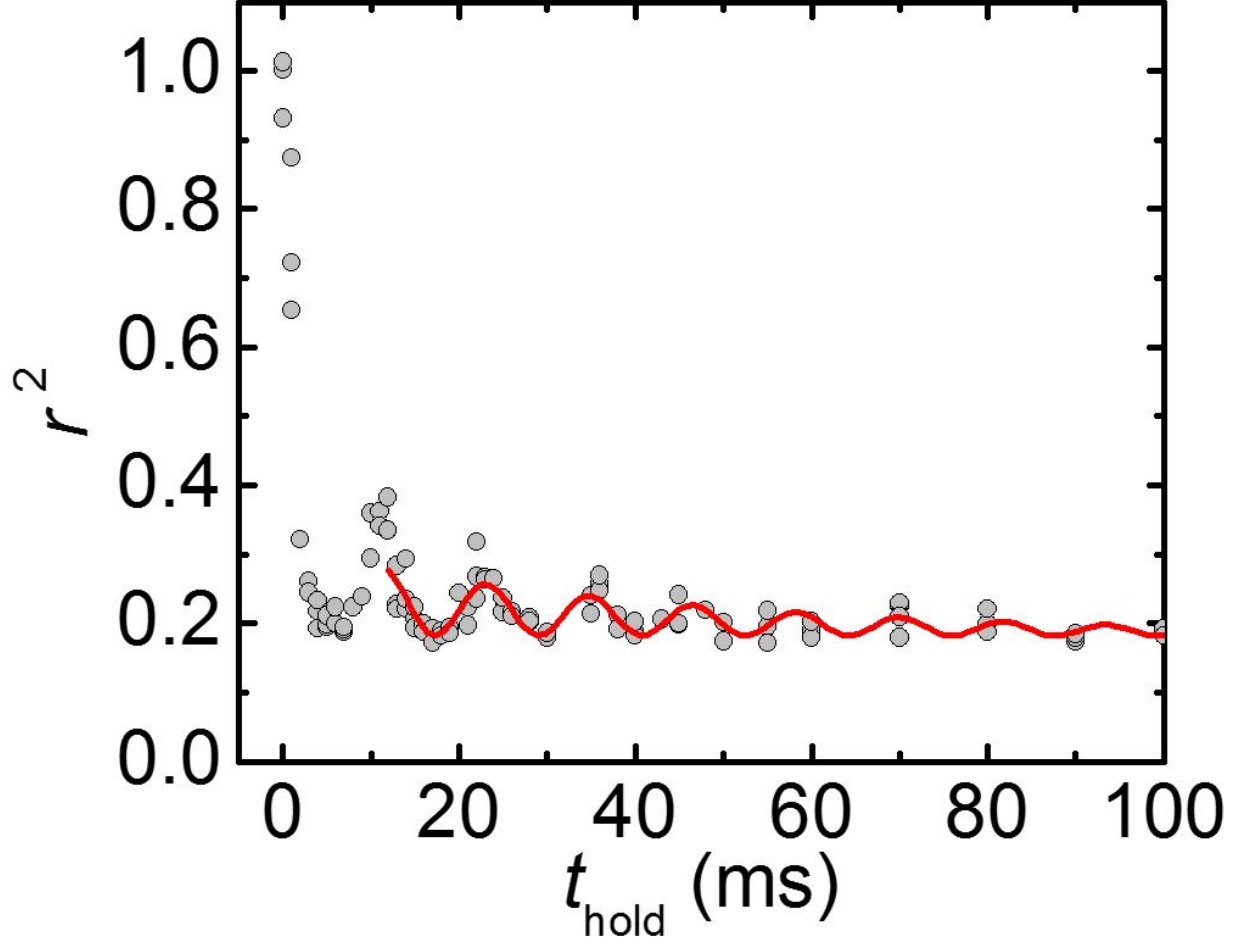

FIG. S3. Mean squared residual  $r^2$  vs. holdtime  $t_{\text{hold}}$  for a thermal gas in a harmonic trap. The vertical axis has been re-scaled. The linear regime is fit to a damped sine-squared function (solid red line).

an exponentially damped oscillatory function indicates that the time constant corresponds to 0.5 collision per particle for a wide range of particle diameters.

We conclude that the measured time constant for relaxation in the dipole trap is consistent with  $N/\Gamma$  within a factor of two. The discrepancy between the measured time constant and the inferred collision rate may arise from systematic uncertainty in the number of particles, trap anharmonicity, and quantum degeneracy effects [4].

## VI. SIMULATION OF COOLING QUASIMOMENTUM

We perform a simple simulation of the potential enhancement in cooling efficiency when more pairs of Raman beams are added to simultaneously remove thermal atoms along one, two, and three lattice vector directions. For the simulation, the cooling sequence is performed iteratively on a 3D quasimomentum distribution based on Eq. (S2). The atom-removal step is modeled via truncation of the quasimomentum distribution beyond a threshold, and the rethermalization step is modeled via calculation of the new equilibrium temperature of the system through energy conservation. A heating rate associated with the laser beams (for  $s = 4 E_R$ ) is also included in the simulation.

In Fig. S4 we show the entropy-per-particle of the gas  $S/N$  versus the number of iterations of the cooling cycle. The 1/2D line (black) corresponds to the case where atoms are removed from one side of the FBZ at a time along one of the lattice vectors, as we have demonstrated experimentally. The 1D line (red) represents the case where atoms on both sides of the FBZ are addressed simultaneously. This can be achieved by using a single pair of Raman beams with a small wavevector  $\Delta k$ , as shown in Fig. S1. The 2D (blue) and 3D (purple) cases refer to the extension of the technique into the orthogonal directions using one and two additional pairs of beams. Fig. S4 shows that the cooling efficiency improves as the technique is extended beyond 1D, and that  $S/N$  converges to zero in a reasonable number of steps.

We conclude that there is no fundamental limitation to cooling via this method for weakly interacting systems. Furthermore, realistic heating rates from the lattice laser beams are not a complication. Ultimately, Pauli blocking [5] and hole heating [6] may limit the lowest temperatures achievable by this method for fermionic atoms. Interaction effects, which will require a more sophisticated analysis, may also introduce difficulties.



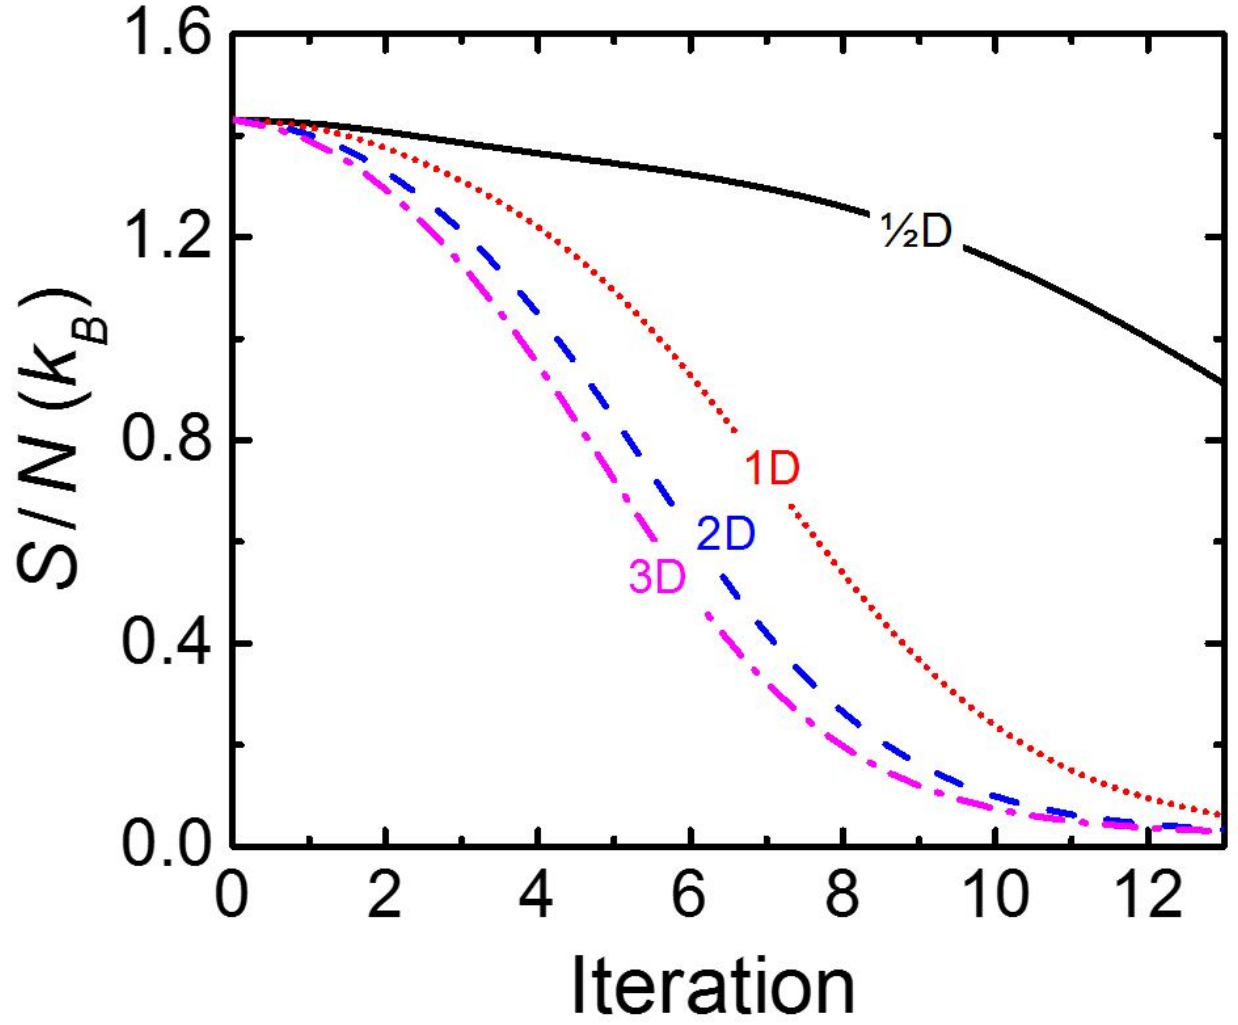

FIG. S4. Simulation of the entropy-per-particle versus number of cooling iterations in 1/2D (black, solid), 1D (red, dotted), 2D (blue, dashed) and 3D (purple, dotted-dashed). The initial atom number is  $N = 1 \times 10^5$  and the initial temperature is  $T = 50$  nK. The initial quasimomentum cutoff is  $0.9 q_B$  and decays exponentially after each iteration. The final cutoff is  $0.02 q_B$ . This strategy has not been optimized for maximum cooling. The estimated heating rate is  $0.15 E_R/s$ .

- 
- [1] D. McKay, M. White, and B. DeMarco, Phys. Rev. A **79**, 063605 (2009).
  - [2] S. Natu, D. McKay, B. DeMarco, and E. Mueller, Phys. Rev. A **85**, 061601 (2012).
  - [3] H. Metcalf and P. van der Straten, *Laser Cooling and Trapping*, Graduate Texts in Contemporary Physics (Springer New York, 1999).
  - [4] S. Koller, A. Groot, R. Duine, H. Stoff, and P. van der Straten, arXiv:1204.6143 (2012).
  - [5] B. DeMarco, S. Papp, and D. Jin, Phys. Rev. Lett. **86**, 5409 (2001).
  - [6] E. Timmermans, Phys. Rev. Lett. **87**, 240403 (2001).
